# Supplementary material for: Ultralow Electron-Surface Scattering in Nanoscale Metals Leveraging Fermi Surface Anisotropy
Source: arXiv:2204.13458 source file (2022-04-28)
Supplement: Supplementary file 1 [file SI.pdf]

# Supplementary Information: Ultralow Electron-Surface Scattering in Nanoscale Metals Leveraging Fermi Surface Anisotropy

Sushant Kumar,[†] Christian Multunas,[‡] Benjamin Defay,[‡] Daniel Gall,[†] and Ravishankar Sundararaman[*,†]

†*Materials Science and Engineering, Rensselaer Polytechnic Institute, Troy, NY 12180, USA*

‡*Physics, Applied Physics and Astronomy, Rensselaer Polytechnic Institute, Troy, NY 12180, USA*

E-mail: sundar@rpi.edu

## Derivation of the resistivity scaling coefficients

### Resistivity scaling coefficient for thin films

We consider steady-state conduction in the $x$-direction through a metallic thin film of thickness $h$ with normal along the $z$-direction. The metal is assumed to be anisotropic with a general band structure. We can describe the conduction using the Boltzmann Transport Equation (BTE) in terms of the distribution function $f_{\mathbf{k}n}(z)$. Note that the distribution function is dependent on both the wave vector $\mathbf{k}$, band index $n$ and height within the film $z$. In steady-state conduction in an infinite area film, there would be no dependence on time or the in-plane directions.

Solving for the distribution function at a specified applied filed $E_x$, we would get the following expression for the average current density:

$$j_x = -\frac{e}{h}\int_0^h dz \sum_n \int_{BZ} \frac{g_s d\mathbf{k}}{(2\pi)^3} \delta f_{\mathbf{k}n}(z) v_{\mathbf{k}n}^x \tag{S1}$$

The BTE in the all-bands relaxation time approximation for this distribution in the interior of the film is:

$$v^z_{\mathbf{k}n} f'_{\mathbf{k}n}(z) + (-eE_x)\frac{\partial f_{\mathbf{k}n}(z)}{\partial p_x} = \frac{f_0(\varepsilon_{\mathbf{k}n}) - f_{\mathbf{k}n}(z)}{\tau_{\mathbf{k}n}} \tag{S2}$$

where $\tau_{\mathbf{k}n}$ is the bulk electron-phonon relaxation time of the electronic state at wave vector $\mathbf{k}$ and band $n$, which may later be simplified to a constant $\tau$ or $\lambda$, if required.

Let us first consider diffuse scattering ($p = 0$) to determine the boundary conditions at $z = 0$ and $z = h$. The simplest model for this would be the assumption that the electrons reflected off the surface completely forget their incident momentum and hence emerge as the thermal distribution (not necessarily isotropic). Therefore,

$$f_{\mathbf{k}n}(0) = f_0(\varepsilon_{\mathbf{k}n}) \ \forall\ \mathbf{k}n \text{ where } v^z_{\mathbf{k}n} > 0 \tag{S3}$$

$$f_{\mathbf{k}n}(h) = f_0(\varepsilon_{\mathbf{k}n}) \ \forall\ \mathbf{k}n \text{ where } v^z_{\mathbf{k}n} < 0 \tag{S4}$$

Finally, we can linearize the BTE to first order in the perturbation due to the electric field in terms of $f_{\mathbf{k}n}(z) = f_0(\varepsilon_{\mathbf{k}n}) + \delta f_{\mathbf{k}n}(z)$. Hence, eq. S2 now becomes:

$$v^z_{\mathbf{k}n}\delta f'_{\mathbf{k}n}(z) + (-eE_x)\frac{\partial[f_0(\varepsilon_{\mathbf{k}n}) + \delta f_{\mathbf{k}n}(z)]}{\partial p_x} = -\frac{\delta f_{\mathbf{k}n}(z)}{\tau_{\mathbf{k}n}} \tag{S5}$$

$$\implies v^z_{\mathbf{k}n}\delta f'_{\mathbf{k}n}(z) + (-eE_x)\frac{\partial f_0(\varepsilon_{\mathbf{k}n})}{\partial \varepsilon_{\mathbf{k}n}} v^x_{\mathbf{k}n} = -\frac{\delta f_{\mathbf{k}n}(z)}{\tau_{\mathbf{k}n}} \tag{S6}$$

Equation S6 is a first order differential equation in $z$ for each $\mathbf{k}n$ with boundary conditions that makes it an initial value problem starting at $z = 0$ when $v^z_{\mathbf{k}n} > 0$ and starting at $z = h$ when $v^z_{\mathbf{k}n} < 0$. By symmetry, the structure of the solution will be identical, just reversed in $z$ starting at the opposite edge. Therefore, let's focus on the $v^z_{\mathbf{k}n} > 0$ contributions, and we can write down the solution for $v^z_{\mathbf{k}n} < 0$ by symmetry:

$$\delta f'_{\mathbf{k}n}(z) + \frac{\delta f_{\mathbf{k}n}(z)}{\tau_{\mathbf{k}n} v^z_{\mathbf{k}n}} + \frac{(-eE_x) f'_0(\varepsilon_{\mathbf{k}n}) v^x_{\mathbf{k}n}}{v^z_{\mathbf{k}n}} = 0 \tag{S7}$$

Substituting $\delta f_{\mathbf{k}n}(z) = g(z) e^{-z/(v^z_{\mathbf{k}n}\tau_{\mathbf{k}n})}$ in the above equation, we get:

$$\delta f_{\mathbf{k}n}(z) = eE_x f'_0(\varepsilon_{\mathbf{k}n}) v^x_{\mathbf{k}n}\tau_{\mathbf{k}n}\left(1 - e^{-z/(v^z_{\mathbf{k}n}\tau_{\mathbf{k}n})}\right) \tag{S8}$$

Using the symmetry, we can complete the solution for both cases:

$$\delta f_{\mathbf{k}n}(z) = \begin{cases} eE_x f'_0(\varepsilon_{\mathbf{k}n}) v^x_{\mathbf{k}n}\tau_{\mathbf{k}n}(1 - e^{-z/(v^z_{\mathbf{k}n}\tau_{\mathbf{k}n})}) & \forall\ v^z_{\mathbf{k}n} > 0 \\ eE_x f'_0(\varepsilon_{\mathbf{k}n}) v^x_{\mathbf{k}n}\tau_{\mathbf{k}n}(1 - e^{(h-z)/(v^z_{\mathbf{k}n}\tau_{\mathbf{k}n})}) & \forall\ v^z_{\mathbf{k}n} < 0 \end{cases}$$

We can combine the two cases above and integrate with respect to $z$:

$$\frac{1}{h}\int dz\,\delta f_{\mathbf{k}n}(z) = eE_x f'_0(\varepsilon_{\mathbf{k}n}) v^x_{\mathbf{k}n}\tau_{\mathbf{k}n}\left(1 - \frac{|v^z_{\mathbf{k}n}|\tau_{\mathbf{k}n}}{h}(1 - e^{-h/(|v^z_{\mathbf{k}n}|\tau_{\mathbf{k}n})})\right) \tag{S9}$$

We can now substitute eq. S9 into eq. S1 and obtain the following expression for conductivity

$$\sigma_x(h) = e^2 \sum_n \int_{BZ} \frac{g_s d\mathbf{k}}{(2\pi)^3} (-f_0'(\varepsilon_{\mathbf{k}n}))(v^x_{\mathbf{k}n})^2 \tau_{\mathbf{k}n} \left(1 - \frac{|v^z_{\mathbf{k}n}|\tau_{\mathbf{k}n}}{h}(1 - e^{-h/(|v^z_{\mathbf{k}n}|\tau_{\mathbf{k}n})})\right) \tag{S10}$$

Next, as we did previously, we assume the electron-phonon relaxation time to be independent of wave vector $\mathbf{k}$ and band number $n$, i.e. $\tau_{\mathbf{k}n} = \tau$. We then have:

$$\sigma_x(h) = e^2 \sum_n \int_{BZ} \frac{g_s d\mathbf{k}}{(2\pi)^3} (-f_0'(\varepsilon_{\mathbf{k}n}))(v^x_{\mathbf{k}n})^2 \tau \left(1 - \frac{|v^z_{\mathbf{k}n}|\tau}{h}(1 - e^{-h/(|v^z_{\mathbf{k}n}|\tau)})\right) \tag{S11}$$

$$\sigma_x(h \gg v_F\tau) \approx e^2 \sum_n \int_{BZ} \frac{g_s d\mathbf{k}}{(2\pi)^3} (-f_0'(\varepsilon_{\mathbf{k}n}))(v^x_{\mathbf{k}n})^2 \tau \left(1 - \frac{|v^z_{\mathbf{k}n}|\tau}{h}\right) \tag{S12}$$

$$= g_1(\hat{x})\tau - g_2(\hat{x},\hat{z})\tau^2/h \tag{S13}$$

where

$$g_1(\hat{x}) \equiv e^2 \sum_n \int_{BZ} \frac{g_s d\mathbf{k}}{(2\pi)^3} (-f_0'(\varepsilon_{\mathbf{k}n}))(v^x_{\mathbf{k}n})^2 \tag{S14}$$

$$g_2(\hat{x},\hat{z}) \equiv e^2 \sum_n \int_{BZ} \frac{g_s d\mathbf{k}}{(2\pi)^3} (-f_0'(\varepsilon_{\mathbf{k}n}))(v^x_{\mathbf{k}n})^2 |v^z_{\mathbf{k}n}| \tag{S15}$$

The above expressions for $g_1(\hat{x})$ and $g_2(\hat{x},\hat{z})$ can be generalized to any current direction $\hat{j}$ and its corresponding normal direction $\hat{n}$ as

$$g_1(\hat{j}) \equiv \sum_b \int_{BZ} \frac{e^2 g_s d\mathbf{k}}{(2\pi)^3} (-f_0'(\varepsilon_{\mathbf{k}b})) \left(\mathbf{v}_{\mathbf{k}b} \cdot \hat{j}\right)^2 \tag{S16}$$

and

$$g_2(\hat{j},\hat{n}) \equiv \sum_b \int_{BZ} \frac{e^2 g_s d\mathbf{k}}{(2\pi)^3} (-f_0'(\varepsilon_{\mathbf{k}b})) \left(\mathbf{v}_{\mathbf{k}b} \cdot \hat{j}\right)^2 |\mathbf{v}_{\mathbf{k}b} \cdot \hat{n}|. \tag{S17}$$

From the above, the resistivity varies as $\rho(h) \approx \rho_0 + g_2(\hat{j},\hat{n})/(g_1(\hat{j})^2 h)$, which is equivalent to the F-S model for single-crystal thin films, but with $\rho_0\lambda$ replaced by

$$r_{\text{film}} \equiv \frac{8 g_2(\hat{j},\hat{n})}{3 g_1(\hat{j})^2}. \tag{S18}$$

## Resistivity scaling coefficient for rectangular wires

Now consider a wire of rectangular cross-section with width $w$ in the $y$ direction and height $h$ in the $z$-direction, with conduction remaining in the $x$-direction. Using the same assumptions above, we once again solve for the first-order change in the electron occupation factors $\delta f_{\mathbf{k}b}(z)$

from the linearized BTE:

$$v^y_{\mathbf{k}n}\frac{\partial\delta f_{\mathbf{k}n}(y,z)}{\partial y}+v^z_{\mathbf{k}n}\frac{\partial\delta f_{\mathbf{k}n}(y,z)}{\partial z}+\frac{\delta f_{\mathbf{k}n}(y,z)}{\tau_{\mathbf{k}n}}=(eE_x)f_0'(\varepsilon_{\mathbf{k}n})v^x_{\mathbf{k}n} \tag{S19}$$

and then determine the average current density using

$$j_x=-e\sum_n\int_{BZ}\frac{g_s d\mathbf{k}}{(2\pi)^3}v^x_{\mathbf{k}n}\frac{1}{wh}\int_0^w dy\int_0^h dz\delta f_{\mathbf{k}n}(y,z) \tag{S20}$$

to determine the resistivity. Diffuse scattering sets the boundary condition $\delta f=0$ on all sides of the rectangle where the velocity $v_{\mathbf{k}n}$ is incoming into the cross-section of the wire. There are four cases based on the signs of $v^y_{\mathbf{k}n}$ and $v^z_{\mathbf{k}n}$ (analogous to the two cases based on the sign of $v_{\mathbf{k}n}$) above. Once again by symmetry, the averaged result will be the same for all sign combinations. Therefore it is sufficient to solve the equation and compute the $yz$-plane average for one of the four quadrants in the $v_yv_z$-plane.

Let's solve the equation for $v_y>0$ and $v_z>0$, dropping $\mathbf{k}n$ subscripts for convenience and denoting the constant RHS as $\dot{f}_0\equiv(eE_x)f_0'(\varepsilon)v_x$:

$$v_y\frac{\partial\delta f}{\partial y}+v_z\frac{\partial\delta f}{\partial z}+\frac{\delta f}{\tau}=\dot{f}_0 \tag{S21}$$

This is an initial value problem starting on the boundary of the rectangle, solved along a line in the direction of the velocity. Let $r$ be the distance along such a line from the initial point, then the above equation reduces to

$$v_\perp\frac{\partial\delta f}{\partial r}+\frac{\delta f}{\tau}=\dot{f}_0 \tag{S22}$$

$$\delta f(r)=\dot{f}_0\tau(1-e^{r/(v_\perp\tau)}) \tag{S23}$$

where $v_\perp\equiv\sqrt{v_y^2+v_z^2}$

We can also perform the integral over the rectangle for the average current by integrating along each such line from boundary to boundary, and then integrating over the incoming edges. If the length of the segment for a specific starting point is $l$, then the total contribution from a specific input boundary point is

$$\delta f_{\text{tot}}=\int_0^l dr\delta f(r)=\dot{f}_0\tau(l-v_\perp\tau(1-e^{-l/(v_\perp\tau)})) \tag{S24}$$

We need to integrate over input points on the two edges $y\in[0,w]$, $z=0$ and $z\in[0,h]$, $y=0$ for the case with $(v_y,v_z)$ in the first quadrant. For a starting point with $y\in[0,w]$, $z=0$, the segment with direction along the velocity must end at either $y'=w$, $z'=(w-y)v_z/v_y$ or $y'=y+hv_y/v_z$, $z'=h$, depending on which intersection happens first. We can determine that simply by computing the lengths of both and finding the shorter. Therefore, the length

of the segment at the input point $y \in [0, w], z = 0$ is:

$$l(y) = \min\left(\sqrt{(w-y)^2\left(1+\left(\frac{v_z}{v_y}\right)^2\right)}, \sqrt{h^2\left(1+\left(\frac{v_y}{v_z}\right)^2\right)}\right) \tag{S25}$$

We can compute the contribution to the current integral from the $y$-edge:

$$\begin{aligned}
I_y &= \frac{v_z}{v_\perp}\int_0^w \mathrm{d}y \dot{f}_0\tau(l(y) - v_\perp\tau(1-e^{-l(y)/(v_\perp\tau)})) \\
&= \frac{v_z}{v_\perp}\int_0^{\max(0, w-hv_y/v_z)} \mathrm{d}y\left(\frac{v_\perp h}{v_z} - v_\perp\tau(1-e^{-h/(v_z\tau)})\right) \\
&= \dot{f}_0\tau\cdot\begin{cases} wh - \frac{h^2 v_y}{2v_z} - hv_y\tau e^{-h/(v_z\tau)} - wv_z\tau(1-e^{-h/(v_z\tau)}) \\ \quad +v_y v_z\tau^2(1-e^{-h/(v_z\tau)}) & , \quad hv_y < wv_z \\ \frac{w^2 v_z}{2v_y} - wv_z\tau + v_y v_z\tau^2(1-e^{-w/(v_y\tau)}), & \quad hv_y > wv_z \end{cases}
\end{aligned}$$

Similarly, we can compute $I_z$ as:

$$I_z = \dot{f}_0\tau\cdot\begin{cases} \frac{h^2 v_y}{2v_z} - hv_y\tau + v_y v_z\tau^2(1-e^{-h/(v_z\tau)}), & \quad hv_y < wv_z \\ wh - \frac{w^2 v_z}{2v_y} - wv_z\tau e^{-w/(v_y\tau)} - hv_y\tau(1-e^{-w/(v_y\tau)}) \\ \quad +v_y v_z\tau^2(1-e^{-w/(v_y\tau)}) & , \quad hv_y > wv_z \end{cases}$$

Adding up the currents $I_y$ and $I_z$ and substituting back, we find the conductivity as:

$$\begin{aligned}
\sigma_x(w,h) &= e^2\sum_b\int_{\mathrm{BZ}}\frac{g_s\mathrm{d}\mathbf{k}}{(2\pi)^3}(-f_0'(\varepsilon_{\mathbf{k}b}))(v^x_{\mathbf{k}b})^2\tau_{\mathbf{k}b} \\
&\quad\times\left[\begin{array}{c} 1-\tau_{\mathbf{k}b}\left(\frac{|v^y_{\mathbf{k}b}|}{w}+\frac{|v^z_{\mathbf{k}b}|}{h}\right)+\frac{2|v^y_{\mathbf{k}b}||v^z_{\mathbf{k}b}|\tau^2_{\mathbf{k}b}}{wh} \\ +\tau_{\mathbf{k}b}\left(\left|\frac{|v^y_{\mathbf{k}b}|}{w}-\frac{|v^z_{\mathbf{k}b}|}{h}\right|-\frac{2|v^y_{\mathbf{k}b}||v^z_{\mathbf{k}b}|\tau_{\mathbf{k}b}}{wh}\right)e^{-\min\left(\frac{h}{|v^z_{\mathbf{k}b}|\tau_{\mathbf{k}b}},\frac{w}{|v^y_{\mathbf{k}b}|\tau_{\mathbf{k}b}}\right)}\end{array}\right]
\end{aligned}$$

For wires that are not much smaller than the mean free path, we can expand:

$$\begin{aligned}
\sigma_x(w,h) &= e^2\sum_b\int_{BZ}\frac{g_s\mathrm{d}\mathbf{k}}{(2\pi)^3}(-f_0'(\varepsilon_{\mathbf{k}b}))(v^x_{\mathbf{k}b})^2\tau_{\mathbf{k}b}\left[1-\tau_{\mathbf{k}b}\left(\frac{|v^y_{\mathbf{k}b}|}{w}+\frac{|v^z_{\mathbf{k}b}|}{h}\right)+O\left(\frac{v_F^2\tau^2}{wh}\right)\right] \\
&\approx g_{1x}\tau-\tau^2\left(\frac{g_{2xy}}{w}+\frac{g_{2xz}}{h}\right) \\
g_{1x} &\equiv e^2\sum_b\int_{\mathrm{BZ}}\frac{g_s\mathrm{d}\mathbf{k}}{(2\pi)^3}(-f_0'(\varepsilon_{\mathbf{k}b}))(v^x_{\mathbf{k}b})^2 \\
g_{2xz} &\equiv e^2\sum_b\int_{\mathrm{BZ}}\frac{g_s\mathrm{d}\mathbf{k}}{(2\pi)^3}(-f_0'(\varepsilon_{\mathbf{k}b}))(v^x_{\mathbf{k}b})^2|v^z_{\mathbf{k}b}| \\
g_{2xy} &\equiv e^2\sum_b\int_{\mathrm{BZ}}\frac{g_s\mathrm{d}\mathbf{k}}{(2\pi)^3}(-f_0'(\varepsilon_{\mathbf{k}b}))(v^x_{\mathbf{k}b})^2|v^y_{\mathbf{k}b}| \\
\frac{\rho_x(w,h)}{\rho_0} &\approx \frac{g_{1x}\tau}{g_{1x}\tau-\tau^2\left(\frac{g_{2xy}}{w}+\frac{g_{2xz}}{h}\right)} \\
&= \left(1-\frac{\tau}{g_{1x}}\left(\frac{g_{2xy}}{w}+\frac{g_{2xz}}{h}\right)\right)^{-1} \\
&= 1+\frac{g_{2xy}\tau}{g_{1x}w}+\frac{g_{2xz}\tau}{g_{1x}h}+O\left(\frac{v_F^2\tau^2}{wh}\right)
\end{aligned}$$

Similar to the case of thin films, we can generalize the above result for current direction $\hat{j}$ and normals $\hat{n}_1$ and $\hat{n}_2$ to get the following expression for resistivity scaling for rectangular wires:

$$r_{\mathrm{wire}}\equiv\frac{8\left(g_2(\hat{j},\hat{n}_1)w+g_2(\hat{j},\hat{n}_2)h\right)}{3g_1(\hat{j})^2(w+h)}, \tag{S26}$$

where $\hat{n}_1$ and $\hat{n}_2$ are the surface normals along the height $h$ and width $w$ directions respectively.

## Data for computed resistivity scaling coefficients

Attached is the data in `.xlsx` format for the computed cohesive energies in eV/atom, the three principal components of the $\rho_0\lambda$ tensor in units of $10^{-16}$ $\Omega\mathrm{m}^2$, worst and best directions of current flow and surface normal ($\hat{j}$ and $\hat{n}$) for thin films and worst and best directions of current flow $\hat{j}$ and normals $\hat{n}_1$ and $\hat{n}_2$ for square wires and the corresponding best and worst $r_{\mathrm{film}}$ and $r_{\mathrm{wire}}$.

## Data for computed electrical resistivity

Attached is the data in `.xlsx` format for the computed electron-phonon mean free paths, relaxation times, Fermi velocities and bulk resistivity for some of the best candidates shortlisted from the above database.

Table S1: Calculated cohesive energy, $E_f$ [eV], number of atoms per unit cell $N_{\mathrm{sites}}$, components of the $\rho_0\lambda$ tensor, best values of $r_{\mathrm{film}}$ and $r_{\mathrm{wire}}$ (in units of $10^{-16}$ $\Omega \mathrm{m}^2$) for metals from the Materials Project database with $r_{\mathrm{wire}} < 3 \times 10^{-16}$ $\Omega \mathrm{m}^2$ ($\sim$ half that of copper).

| MP-ID | Formula | $N_{\mathrm{sites}}$ | $E_f$ | $(\rho_0\lambda)_{xx}$ | $(\rho_0\lambda)_{yy}$ | $(\rho_0\lambda)_{zz}$ | $r_{\mathrm{film}}$ | $r_{\mathrm{wire}}$ |
|---|---|---|---|---|---|---|---|---|
| mp-1220023 | OsRu | 2 | 7.43 | 5.88 | 5.88 | 4.22 | 2.97 | 2.99 |
| mp-999376 | NbPt | 4 | 6.62 | 10.81 | 9.52 | 6.77 | 2.42 | 2.98 |
| mp-1228631 | $B_4OsW$ | 6 | 7.20 | 19.17 | 19.17 | 6.12 | 2.94 | 2.93 |
| mp-15297 | $Hf_6NiSb_2$ | 9 | 5.65 | 82.67 | 82.67 | 7.21 | 2.86 | 2.86 |
| mp-12760 | $Zr_6Al_2Co$ | 9 | 5.48 | 23.71 | 23.71 | 6.74 | 2.80 | 2.79 |
| mp-13092 | $Zr_6Al_2Ni$ | 9 | 5.44 | 25.32 | 25.32 | 6.26 | 2.76 | 2.78 |
| mp-20318 | $Mn_2B$ | 6 | 4.87 | 12.25 | 12.25 | 4.03 | 2.72 | 2.72 |
| mp-1079597 | ScGeRh | 9 | 5.30 | 50.89 | 50.81 | 6.88 | 2.72 | 2.71 |
| mp-1773 | $ReB_2$ | 6 | 7.15 | 17.58 | 17.58 | 6.33 | 2.69 | 2.70 |
| mp-20536 | CoSn | 6 | 4.14 | 51.19 | 51.19 | 5.90 | 2.60 | 2.61 |
| mp-22191 | HfFeGe | 9 | 5.32 | 45.36 | 45.36 | 7.56 | 2.46 | 2.47 |
| mp-570713 | TiAlPt | 6 | 5.46 | 17.57 | 17.57 | 4.96 | 2.43 | 2.44 |
| mp-1079155 | $Hf_6Al_2Pt$ | 9 | 5.86 | 37.58 | 37.53 | 6.39 | 2.37 | 2.37 |
| mp-7804 | $HfCo_3B_2$ | 6 | 6.15 | 24.70 | 24.70 | 5.28 | 2.34 | 2.34 |
| mp-1606 | $NbAu_2$ | 3 | 4.35 | 28.50 | 28.50 | 9.45 | 2.25 | 2.27 |
| mp-20826 | CuTe | 4 | 2.97 | 124.46 | 14.84 | 8.95 | 1.35 | 2.24 |
| mp-10059 | $ZrCo_3B_2$ | 6 | 6.09 | 23.60 | 23.60 | 4.75 | 2.22 | 2.22 |
| mp-1080489 | HfGeRu | 9 | 6.20 | 54.92 | 54.87 | 7.40 | 2.18 | 2.19 |
| mp-5019 | $YCo_3B_2$ | 6 | 5.64 | 27.96 | 27.96 | 5.07 | 2.14 | 2.15 |
| mp-1080817 | NbFeB | 9 | 6.41 | 32.73 | 32.68 | 5.52 | 2.09 | 2.10 |
| mp-16305 | ScPRu | 9 | 5.78 | 83.82 | 83.82 | 6.61 | 2.06 | 2.05 |
| mp-1025045 | TiGaPd | 6 | 4.37 | 20.82 | 20.82 | 4.90 | 2.03 | 2.04 |
| mp-1095196 | HfGeOs | 9 | 6.53 | 43.58 | 43.57 | 7.75 | 2.03 | 2.03 |
| mp-22662 | TiGaPt | 6 | 5.10 | 18.71 | 18.71 | 4.71 | 2.02 | 2.02 |
| mp-1078884 | HfSiRu | 9 | 6.66 | 49.06 | 49.05 | 7.01 | 2.01 | 2.02 |
| mp-4938 | $ScCo_3B_2$ | 6 | 5.71 | 28.13 | 28.13 | 4.79 | 1.97 | 1.98 |
| mp-1079323 | HfSiOs | 9 | 7.05 | 38.97 | 38.91 | 7.24 | 1.97 | 1.97 |
| mp-1091395 | ZrGeOs | 9 | 6.47 | 41.26 | 41.25 | 7.83 | 1.96 | 1.96 |
| mp-7544 | ZrSiRu | 9 | 6.57 | 44.70 | 44.70 | 7.07 | 1.92 | 1.92 |
| mp-1080089 | TaFeB | 9 | 6.87 | 35.95 | 35.92 | 5.44 | 1.89 | 1.90 |

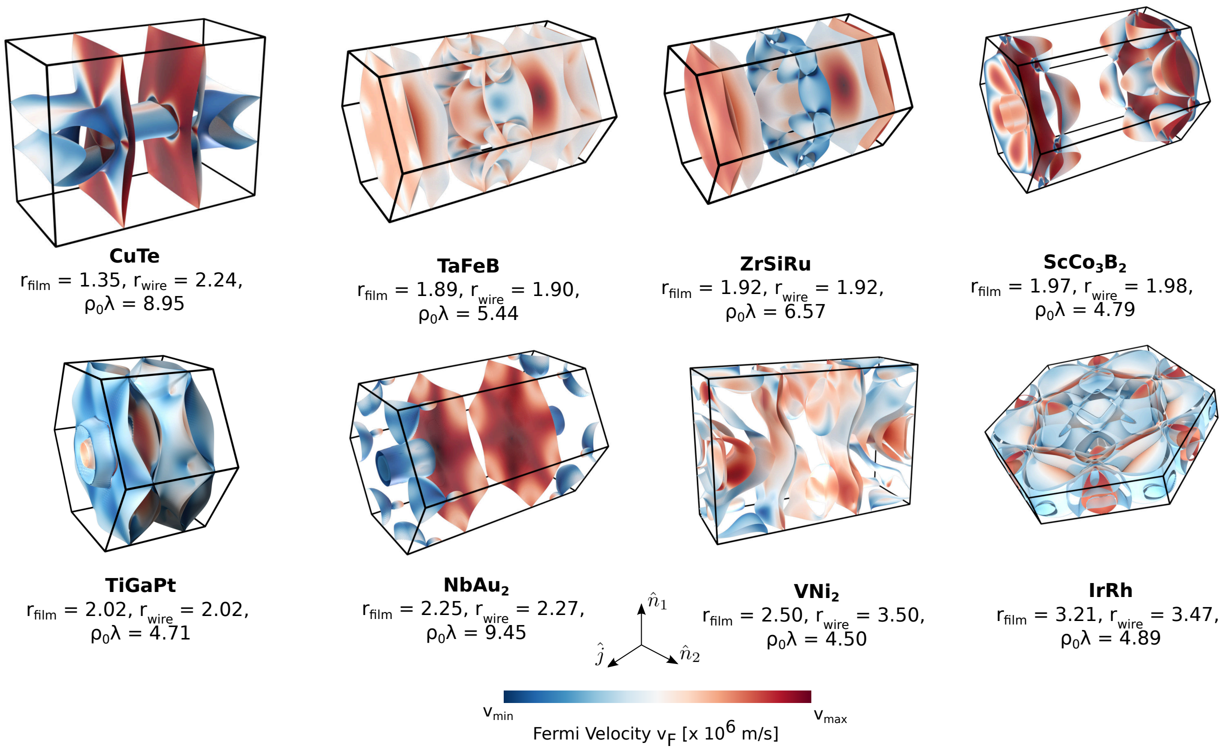


Figure S1: Fermi surfaces of the some of the best nanoscale conductors, shortlisted by resistivity scaling coefficients $r_{\text{film}}$ and $r_{\text{wire}}$ (in $10^{-16}$ $\Omega\text{m}^2$). All tend to have flat surfaces perpendicular to the best direction of current flow, leading to large Fermi velocities directed along the transport direction $\hat{j}$ and much smaller velocity components along the surface normal $\hat{n}_1$ and side wall $\hat{n}_2$ directions.

Table S2: Comparison of values of $\rho_0\lambda$ computed using JDFTx with the ones calculated by Gall.[1] For most metals, the computed values are within 5% of the ones found in the literature.

| Element | Structure | $\rho_0\lambda$ ($10^{-16}$ $\Omega$m$^2$)[1] | $\rho_0\lambda$ ($10^{-16}$ $\Omega$m$^2$) [This work] | Error % |
|---|---|---|---|---|
| Ag | FCC | 8.46 | 8.76 | -3.5 |
| Cu | FCC | 6.70 | 6.73 | -0.45 |
| Au | FCC | 8.35 | 8.72 | -4.4 |
| Rh | FCC | 3.23 | 3.32 | -0.40 |
| Ir | FCC | 3.69 | 3.73 | -2.8 |
| Ni | FCC | 4.07 | 3.78 | -1.1 |
| W | BCC | 8.20 | 8.12 | 1.0 |
| Mo | BCC | 5.99 | 5.98 | 0.17 |
| Zn | HCP | 10.3/8.1 | 9.80/8.83 | 4.9/-9.0 |
| Co | HCP | 7.31/4.82 | 7.16/5.02 | 2.1/-4.1 |
| Cd | HCP | 12.6/11.3 | 12.39/11.76 | 1.7/-4.1 |
| Ru | HCP | 5.14/3.87 | 5.27/3.87 | -2.6/0.0 |
| Os | HCP | 6.41/4.33 | 6.58/4.41 | -2.7/-1.9 |

# References

(1) Gall, D. Electron Mean Free Path in Elemental Metals. *J. Appl. Phys.* **2016**, *119*, 085101.
